# Supplementary material for: Backdoors Stuck At The Frontdoor: Multi-Agent Backdoor Attacks That Backfire
Source: arXiv:2201.12211 source file (2022-01-28)
Supplement: Supplementary file 2 [file 8.uninserted_appendix.tex]

\section{Uninserted Appendix}

{\color{blue}
\begin{itemize}
    \item Explain why converge to 0.1
    
    For poisoned labels, this can be explained by the overlapping case where a poisoned label is identical to the clean label for a randomly sampled input. For clean labels, this can be explained as random guessing by the model across 10 classes.  
    
    The distribution of target poison labels may or may not be random.
    The distribution of clean labels are random, as we randomly sample inputs from the attacker's private dataset to re-assign clean labels to target poison labels.
    As all our evaluation datasets have 10 classes, this means $\frac{1}{10}$ of all backdoored inputs have target poison labels equivalent to clean labels.
    % Hence, the lower bound for both Attack Success Rate (accuracy w.r.t. poisoned labels) and Standard Accuracy (accuracy w.r.t. clean labels) are both 0.1.
    We only tabulate the raw accuracy w.r.t. poisoned labels;
    a more reflective attack success rate would be ($\texttt{Acc w.r.t. poisoned labels}-0.1$).
    
    \item 
    
\end{itemize}
}

\subsection{Subnetwork gradient selection w.r.t. $\mathcal{L}$}
\label{r2.2}

Given fixed model capacity, 
% if the number of attackers $N$ is very large resulting in many candidate subnetworks, not all of them can be inserted into $\theta$.
$\theta$ can only include a limited number of subnetworks, and this number can depends ultimately by each subnetwork carries information that can reduce loss for multiple backdoored sets of inputs (transferability).
% We can approximate this transferability by studying how the loss changes with respect to this subnetwork and 2 sets of inputs. 
% There is insufficient results that indicate a precise form of measurement of this transferability in terms of the weight sub-matrice values in the model weights and computing distance scores between subnetworks. 
% 
\begin{equation}
\small
\begin{split}
& \sum_{x, y}^{\mathbb{D} \setminus D_i} 
\mathcal{L}(\theta + \sum \phi_{n}^{\textnormal{backdoor}}; x^{\textnormal{clean}}, y^{\textnormal{clean}}) \\ + & \sum_{i}^{N} \sum_{x, y}^{D_i} \mathcal{L}(\theta + \sum \phi_{n}^{\textnormal{backdoor}}; x^{\textnormal{poison}}, y^{\textnormal{poison}})
\\ < 
& \sum_{x, y}^{\mathbb{D} \setminus D_i}  \mathcal{L}(\theta; x^{\textnormal{clean}}, y^{\textnormal{clean}}) \\ + & \sum_{i}^{N} \sum_{x, y}^{D_i} \mathcal{L}(\theta; x^{\textnormal{poison}}, y^{\textnormal{poison}})
\nonumber
\end{split}
\tag{16}
% \label{equation:4}
\end{equation}
Compared to the single-agent attack, the information:capacity ratio per backdoor subnetwork is diluted. We can infer this from Eqt \ref{equation:4} (a multi-agent extension of Eqt \ref{equation:2a}), where $N$ subnetworks are required to carry information to compute correct predictions for all $N$ backdoored sets compared to 1 in single-attacker scenario. 
The loss optimization procedure (Eqt \ref{equation:4}) determines the selection of subnetworks that should be selected to minimize total loss over the joint dataset:
% The subnetwork would be updated based on update condition (\ref{equation:1}), where 
the insertion of the subnetwork would be rejected if $\textnormal{LHS} > \textnormal{RHS}$ (\ref{equation:4}). 
It implicitly determines which backdoored private datasets to ignore with respect to loss optimization, which we reflect in Eqt \ref{equation:7}.
% The loss difference is larger in $\textnormal{LHS}$ (\ref{equation:4}) than $\textnormal{RHS}$ (\ref{equation:4}), hence if it is a question of including all the backdoor subnetworks or none at all, 
We detail our steps in induction and inference of this section in Appendix \ref{aSub}.
\begin{equation}
\small
\begin{split}
\{ \varepsilon \}^{*} := 
\argmin_{\{ \varepsilon \}}
\bigg[
& \mathbf{sign}(\frac{\partial \mathcal{L}(\mathbf{x}, y)}{\partial \theta})
\\ +
\sum_{\varepsilon}^{\{ \varepsilon \}}
& \mathbf{sign}(\frac{\partial \mathcal{L}(\varepsilon, y)}{\partial \theta})
 \equiv -(1 + |\{ \varepsilon \}|)
\bigg]
\nonumber
\end{split}
\tag{17}
% \label{equation:7}
\end{equation}
% 
% The above assumes thus far that only 1 subnetwork can be inserted (when in practice multiple subnetworks may be insertable depending on the transferabiltiy of the candidate subnetworks against the sub-datasets), or that all subnetworks must be inserted or none at all. 
With {\small $\mathbf{sign}(x)=\begin{cases} +1 \phantom{=} \textnormal{for } x \geq 0 \\ -1 \phantom{=} \textnormal{for } x < 0 \end{cases}$}, 
% condition \ref{equation:2d} must be satisfied to accept the candidate subnetwork. 
we extend update condition (\ref{equation:4}) into a subnetwork set optimization procedure (Eqt \ref{equation:7}), where loss optimization attempts to determine a set of backdoor subnetworks that can minimize the total loss over as many private datasets. 
To make a backdoor subnetwork more salient with respect to procedure (\ref{equation:7}), an attacker could (i) increase their individual $p_n$, (ii) have similar backdoor patterns and target poison labels as other attackers (or any other form of cooperative behavior).
We empirically show this in Experiments \ref{3.4}.

With respect to Experiments \ref{3.3}, adversarial perturbations work because they re-use existing subnetworks in $\theta$ (i.e. $\phi^{\textnormal{clean}}$) without the need to insert a new one.
Stylized perturbations can be decomposed into style and content features; the content features may have transferability against unstylized content features thus there may be no subsequent change to $\phi^{\textnormal{clean}}$, though the insertion of a new $\phi^{\textnormal{style}}$ faces a similar insertion obstacle as $\phi^{\textnormal{backdoor}}$.

Backdoor subnetworks can have varying distances from each other (e.g. depending on how similar the backdoor trigger patterns and corresponding target poison labels are).
Measuring the distance between subnetworks would be one way of testing whether a subnetwork carries transferable features for multiple sub-datasets, as at least in the backdoor setting each candidate subnetwork tends to be mapped to a specific sub-dataset. 
Based on Experiments \ref{}, 
we observe that the parameters diverge as $N$ increase per layer, indicating the low likelihood that at scale a large number of random trigger patterns can share common transferable backdoors.
In other words, this supports the notion that each subnetwork is relatively unique for each trigger pattern and share low transferability across a set of private datasets $|| \phi_i(x) - \phi_j(x) ||_2^2 > 0$.

Unused text:
\begin{enumerate}
    \item 
\end{enumerate}

% Capacity
\begin{table*}
	\begin{minipage}{0.32\textwidth}
		\centering
		\resizebox{\textwidth}{!}{
        \begin{tabular}{|lcc|}
        \hline
        Name 
        & \textit{Number of parameters}            
        & \textit{Ratio w.r.t ResNet18}               
        \\ \hline
        
         \tikz\draw[smallcnn,fill=smallcnn] (0,0) circle (.5ex); SmallCNN
        & {\color{black} 15,722}
        & {\color{black} 0.0014}
        \\ \hline
        
         \tikz\draw[resnet9,fill=resnet9] (0,0) circle (.5ex); ResNet9
        & {\color{black} 7,756,554}
        & {\color{black} 0.6936}
        \\ \hline
        
         \tikz\draw[resnet18,fill=resnet18] (0,0) circle (.5ex); ResNet18
        & {\color{black} 11,181,642}
        & {\color{black} 1.0000}
        \\ \hline
        
         \tikz\draw[resnet34,fill=resnet34] (0,0) circle (.5ex); ResNet34
        & {\color{black} 21,289,802}
        & {\color{black} 1.9040}
        \\ \hline
        
         \tikz\draw[resnet50,fill=resnet50] (0,0) circle (.5ex); ResNet50
        & {\color{black} 23,528,522}
        & {\color{black} 2.1042}
        \\ \hline
        
         \tikz\draw[resnet101,fill=resnet101] (0,0) circle (.5ex); ResNet101
        & {\color{black} 42,520,650}
        & {\color{black} 3.8027}
        \\ \hline
        
         \tikz\draw[resnet152,fill=resnet152] (0,0) circle (.5ex); ResNet152
        & {\color{black} 58,164,298}
        & {\color{black} 5.2018}
        \\ \hline
        
         \tikz\draw[wide_resnet50_2,fill=wide_resnet50_2] (0,0) circle (.5ex); W-ResNet50
        & {\color{black} 66,854,730}
        & {\color{black} 5.9790}
        \\ \hline
        
         \tikz\draw[wide_resnet101_2,fill=wide_resnet101_2] (0,0) circle (.5ex); W-ResNet101
        & {\color{black} 124,858,186}
        & {\color{black} 11.1664}
        \\ \hline
        
         \tikz\draw[vgg,fill=vgg] (0,0) circle (.5ex); VGG
        & {\color{black} 128,812,810}
        & {\color{black} 11.5200}
        \\ \hline
        
        \end{tabular}
        }
	\end{minipage}\hfill
	\begin{minipage}{0.32\textwidth}
		\centering
		\includegraphics[width=\textwidth]{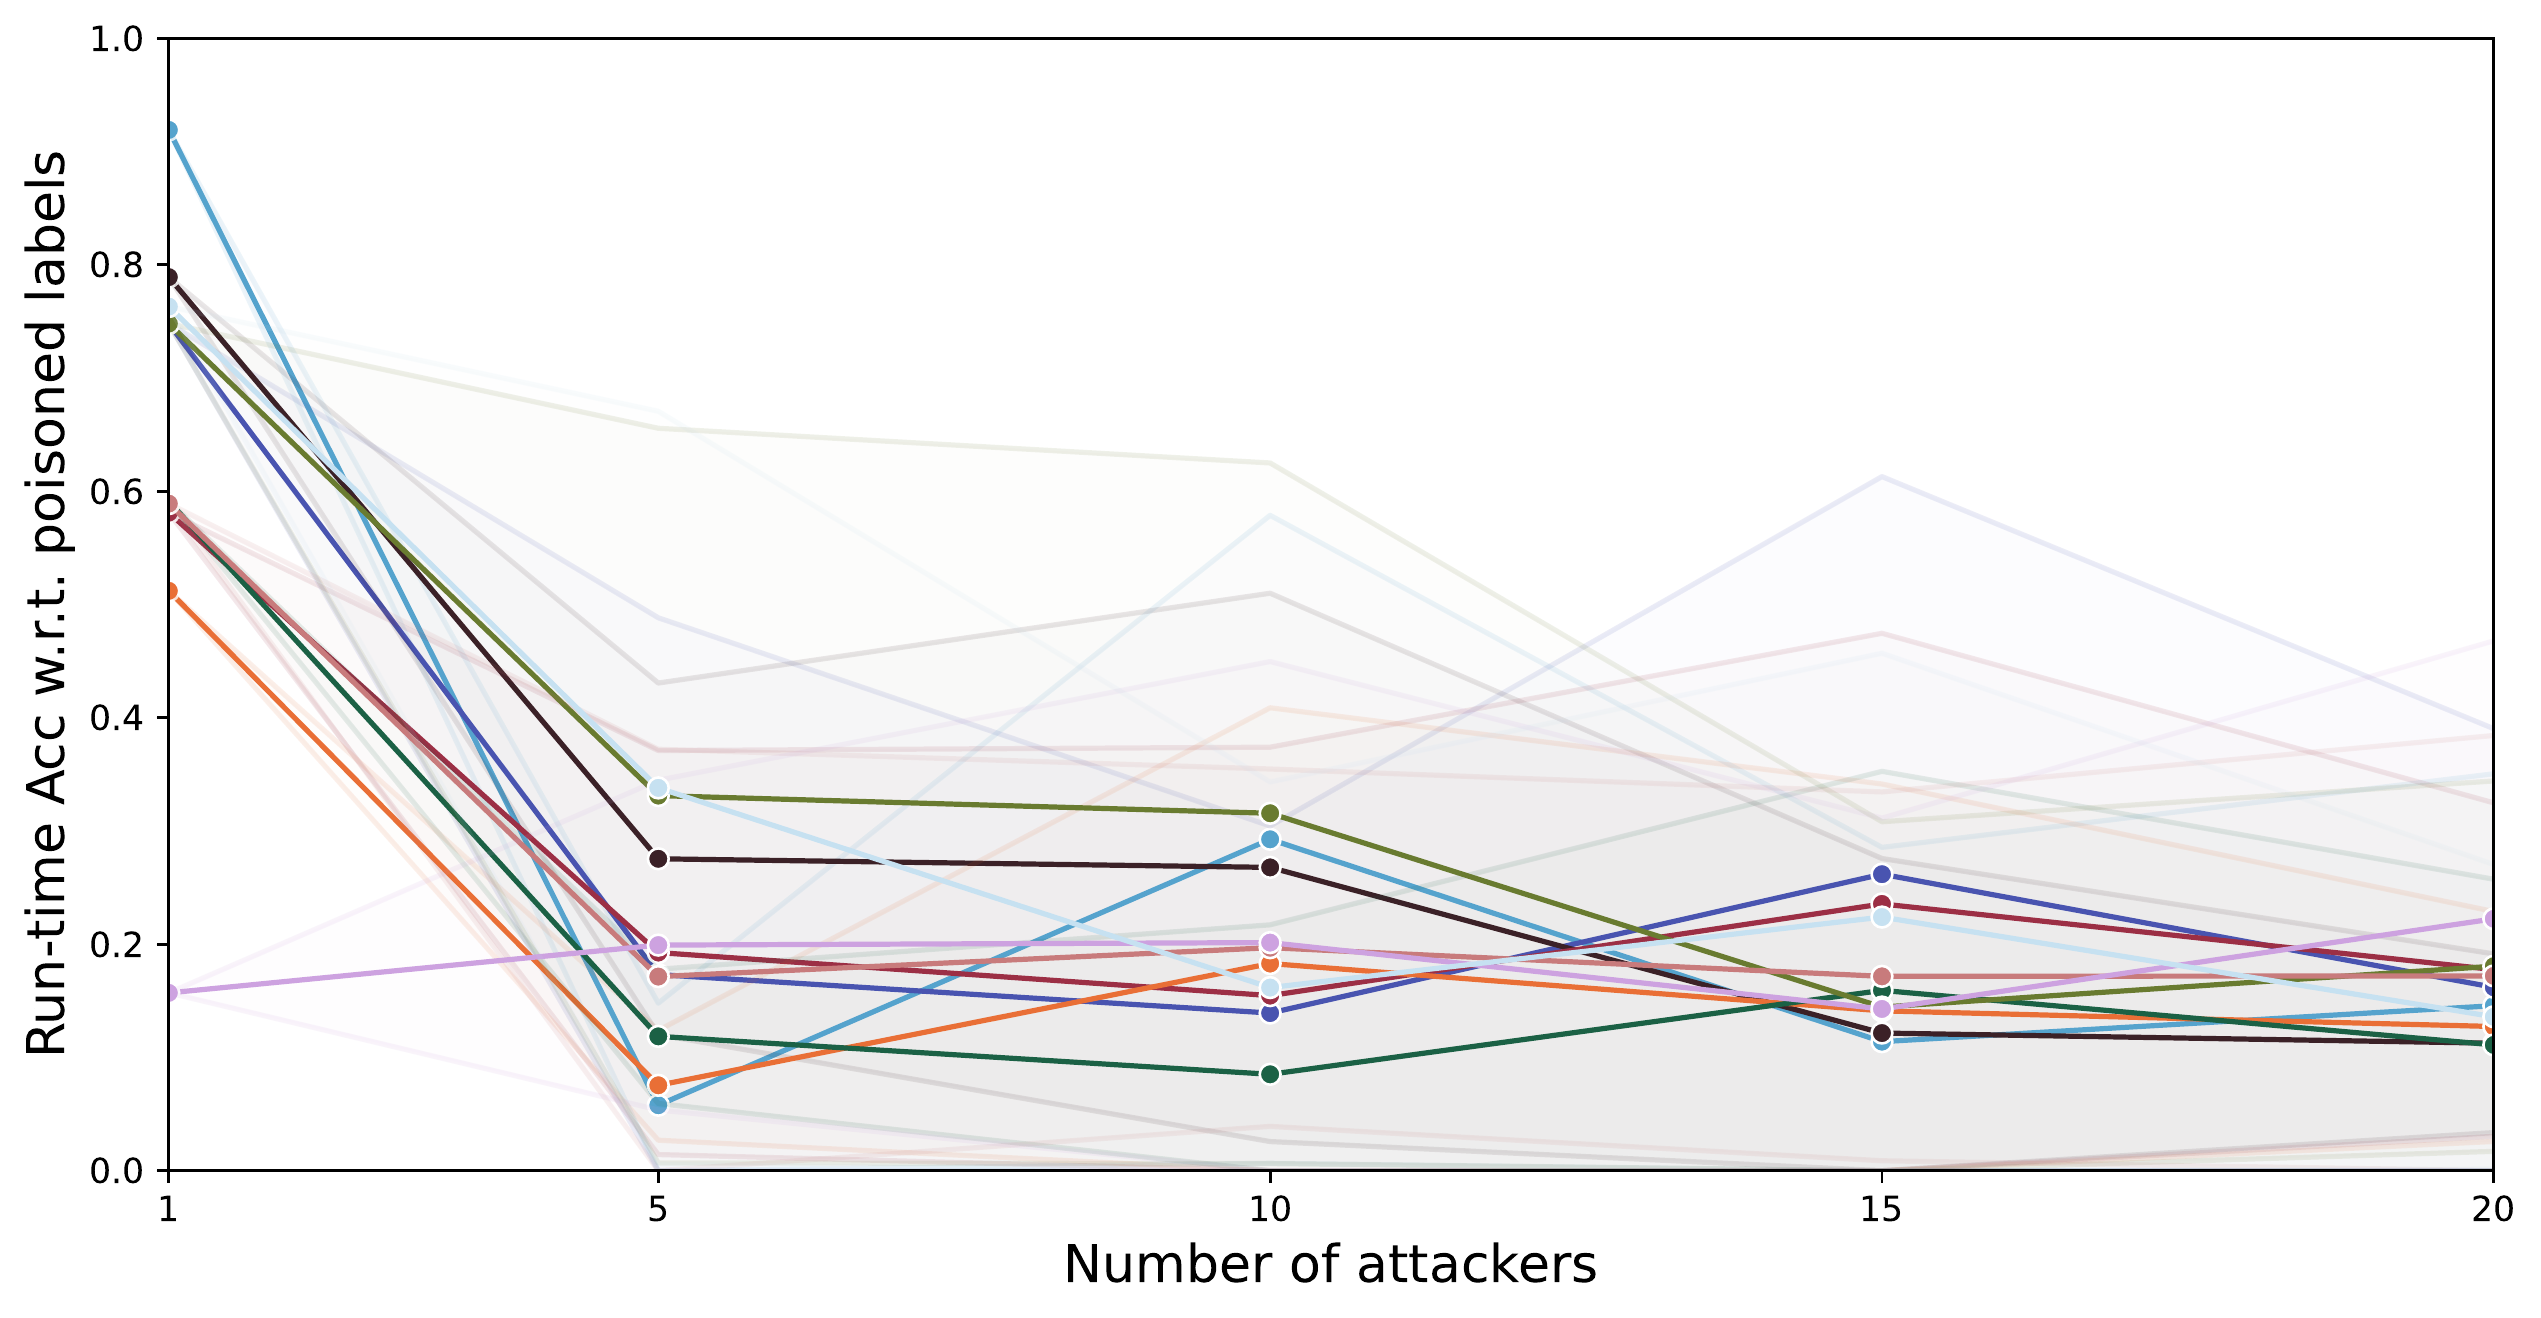}
	\end{minipage}
	\begin{minipage}{0.32\textwidth}
		\centering
		\includegraphics[width=\textwidth]{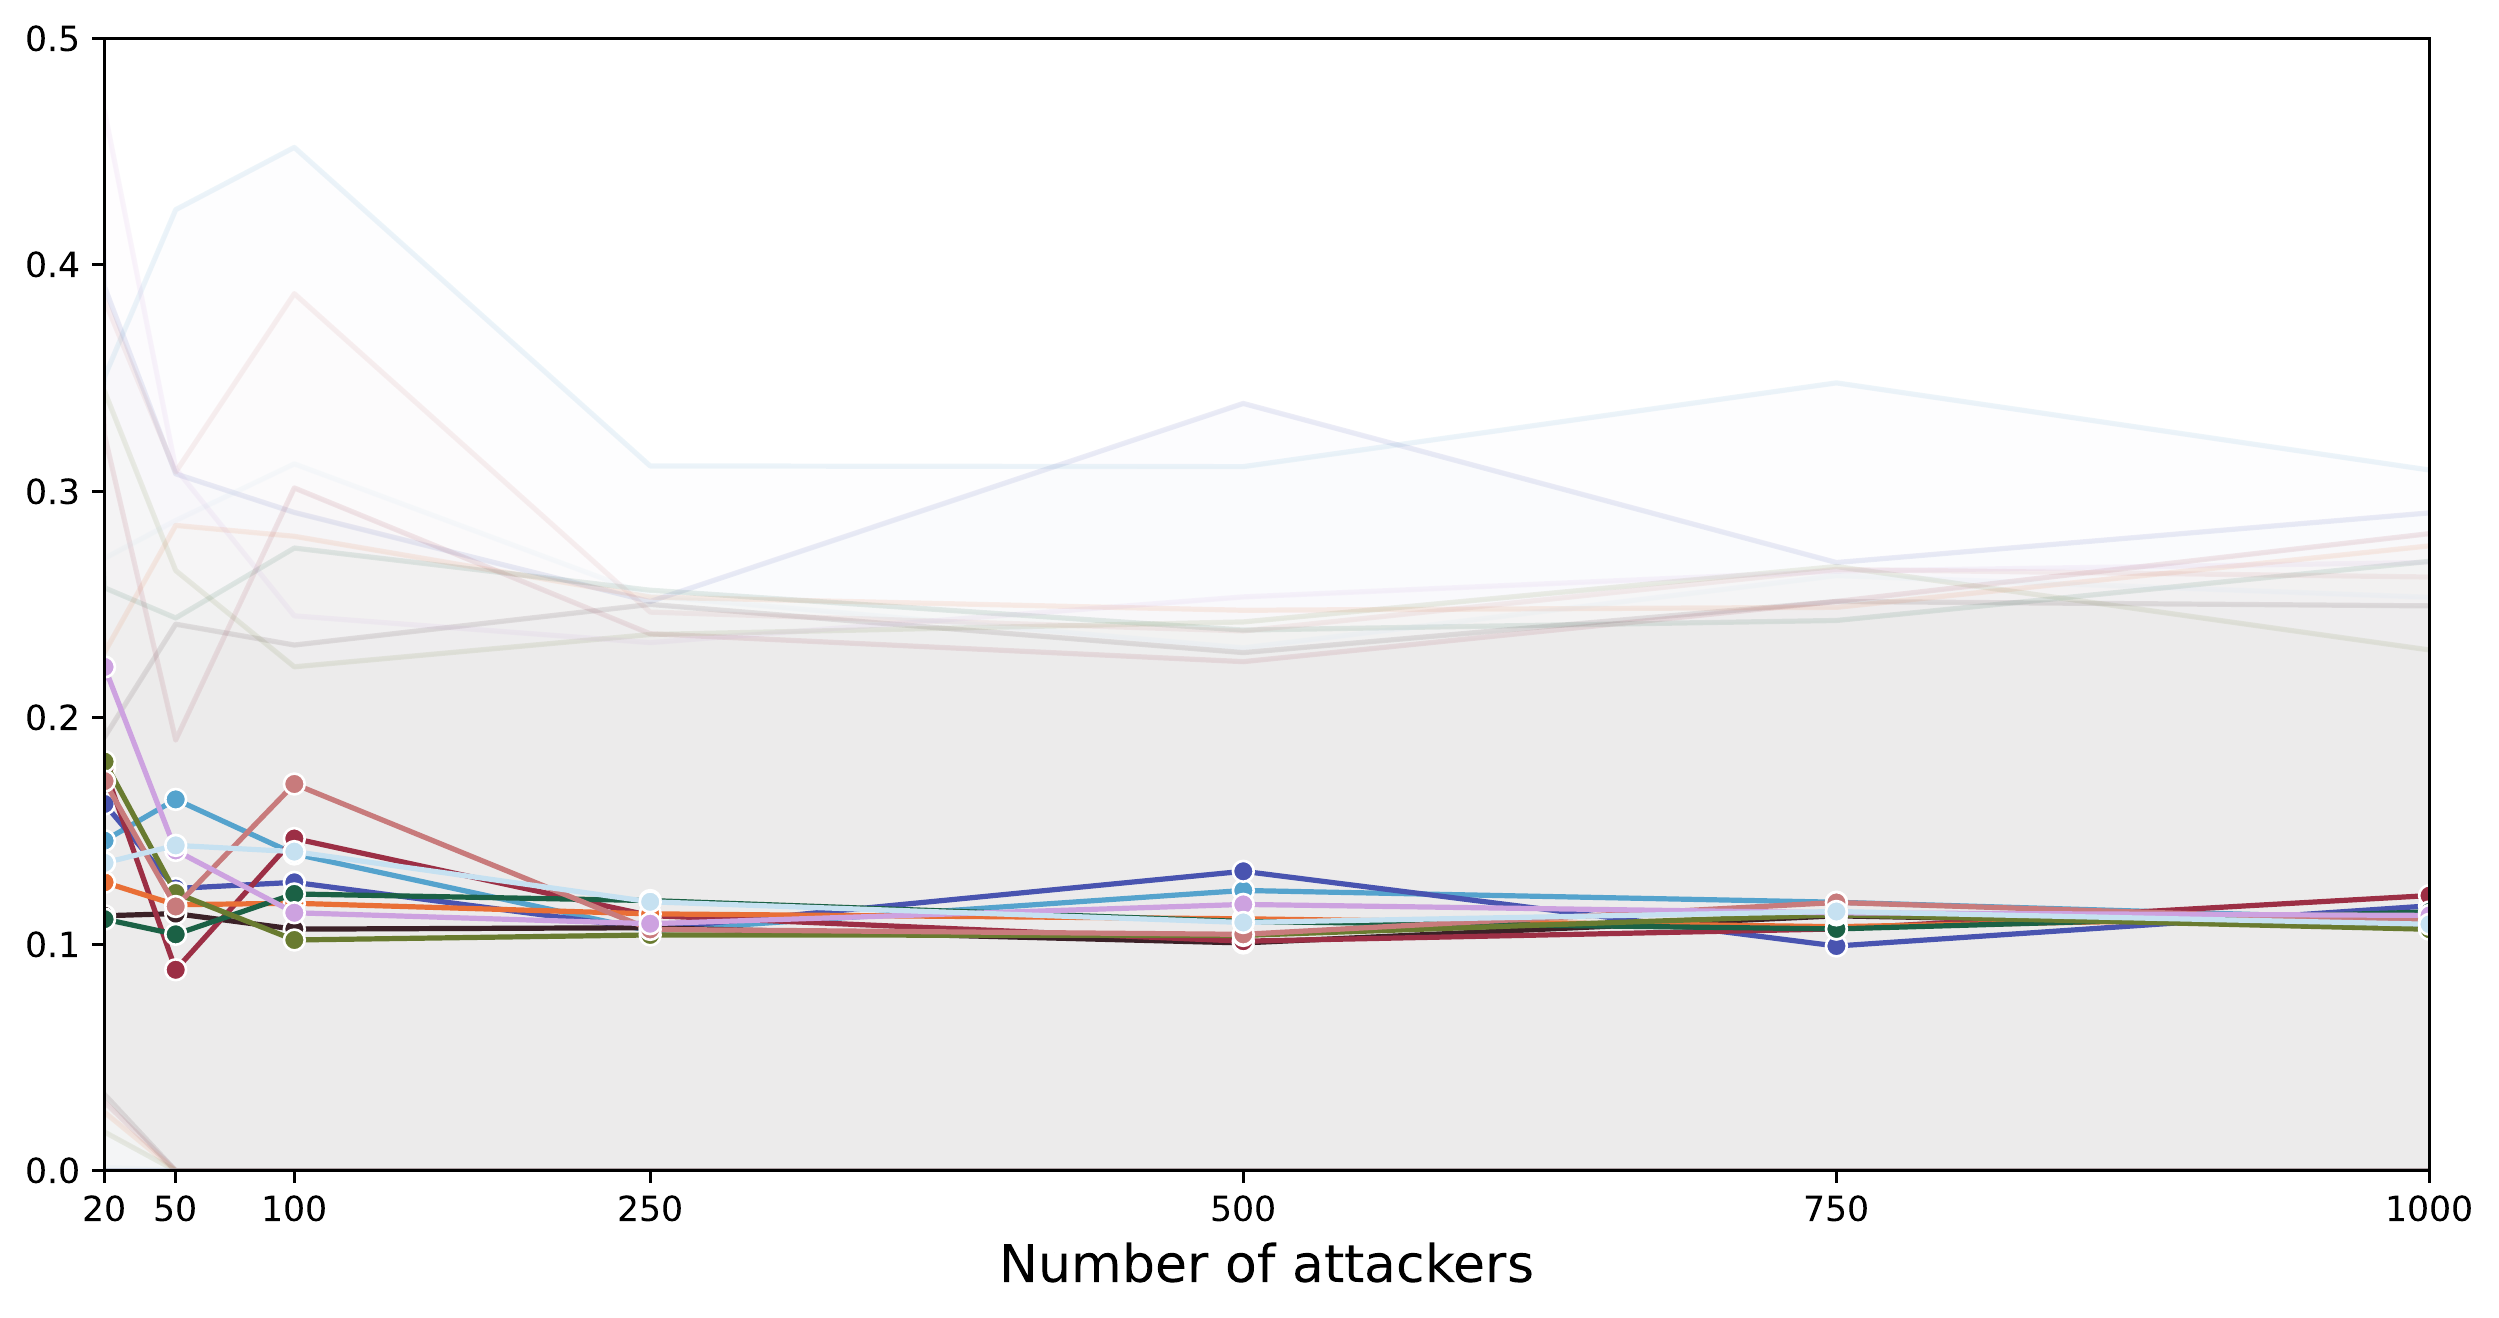}
	\end{minipage}
	\caption{A table beside a figure}
	\label{tab:capacity}
\end{table*}

\subsubsection{Adversarial-Backdoor shift comparison}
% Show they are the same

{\color{blue}

\noindent\textbf{Definition 1: Distribution Shift. }
A \textit{feature} is defined here as a collection of sub-inputs (e.g. pixels, word embeddings) that are relevant to class/label $Y$.
The \textit{distribution} refers to the distribution of features relevant to class/label $Y$.
We classify two types of distributions: (i) the \textit{train-time} distribution originates from the training dataset, and (ii) the \textit{test-time} distribution originates from the source of test inputs that need to be evaluated. 
We denote \textbf{\textit{distribution shift}} as the change or shift or divergence between the train-time distribution and test-time distribution. 

Let $\mathcal{X}$ be the input space and $\mathcal{Y} = {1, 2, . . . , k}$ the output space. 
We denote train-time distribution by the probability density function $p^{train}(x) = \{p^{train}_{Y=Y_i}\}$ $\forall Y_i \in \mathcal{Y}$.
We denote test-time distribution by the probability density function $p^{test}(x) = \{p^{test}_{Y=Y_i}\}$ $\forall Y_i \in \mathcal{Y}$.
We denote a distance metric $d(p(\cdot), p(\cdot))$ such that distribution shift is measured as the divergence between the train-time and test-time distributions $d(p^{train}(x), p^{test}(x)) \geqslant 0$.

Distribution shift is discussed in literature distinctly and sometimes independently in its different forms, such as label shift (adversarial attacks, backdoor attacks), domain shift, task shift, agent shift, etc. We show they share similar properties to unify them under the concept of distribution shift.

\noindent\textbf{Definition 2: Label Shift. } 
\textit{Label shift} is a distribution shift setting in which the labels $Y$ cause the features in $X$, i.e. the feature distribution remains the same, but the label distribution varies \citep{garg2020unified}.
It is the overlap in features between the feature distributions of multiple classes/labels. When a feature from an opposing class $Y_0$ manifests in an input $X_{Y_1}$ of a different class $Y_1$ during test-time, the model tends to misclassify the input $X_{Y_1}$ as $Y_0$. 

Let $\mathbf{P}_{Y=s}, \mathbf{P}_{Y=t} : \mathcal{X} \times \mathcal{Y} \rightarrow [0, 1]$ be the source (e.g. class/label $Y=Y_0$) and target distributions (e.g. class/label $Y=Y_1$) where $s \neq t$. Let $p_{Y=s}$ and $p_{Y=t}$ denote the corresponding probability density functions. 
We construct a base learner function $\widehat{f}: \mathcal{X} \mapsto \mathcal{Y}$, where $\widehat{f}$ is trained to approximate the true probability function $f^{*}(x):=p_{Y}(x)$.
If $f$ accepts specific weights/parameters $\theta$ as an argument to predict label $y$ from input $x$, we denote it as $y = f(\theta; x)$.
We assume here that function $\widehat{f}$ approximates a set of probability density functions for each class/label $\{p_{Y=Y_i}\} \in \widehat{f}$ $\forall Y_i \in \mathcal{Y}$.
In this text, $p(x)$ refers to the collection of probability density functions for each class/label $p(x) = \{p_{Y=Y_i}\}$ $\forall Y_i \in \mathcal{Y}$.
% Under label shift, the label distribution $p(y)$ might change but the class-conditional distributions $p(x|y)$ do not.
$p_{s}(x|s)$ denotes the probability that an input $x$ with ground truth label $s$ is predicted to return the label $s$. 
$p_{t}(x|s)$ denotes the probability that an input $x$ with ground truth label $s$ is predicted to return the label $t$. 
We possess labeled data ${(x_0, y_0),(x_1, y_1), . . . ,(x_n, y_n)}$.
Label shift is defined as the state where $p_{Y=s}(x|Y=s)=p_{Y=t}(x|Y=s)$.

\noindent\textbf{Observation 1: Adversarial and backdoor perturbations can be reformulated as label shift. }
An \textit{adversarial attack} is a test-time distribution shift setting where an attacker introduces a small, imperceptible perturbation $\epsilon$ to a clean input $X$ such that $f(X) \neq f(X+\epsilon)$. In the Fast Gradient Sign Method \citep{goodfellow2015explaining}, the attacker constructs adversarial samples with respect to the defender's gradients: $\arg\min_{\epsilon} X + \epsilon \textnormal{sign}(\nabla_X \mathcal{L}(X, Y))$, where $\mathcal{L}(X, Y)$ is the loss incurred in classifying input $X$ with label $Y$, and $\nabla_X \mathcal{L}(X, Y)$ is the gradient.

A \textit{backdoor attack} is a train-time distribution shift setting where an attacker introduces a perturbation $\epsilon$ to a set of inputs $X$ with a target label $Y^{*}$, and contributes this perturbed set of inputs to a victim's training set \textbf{$V$}. 
The attacker determines a poison rate $\rho$, which is the proportion of the victim's training set that contains inputs with perturbation $\epsilon$. 
In BadNet \citep{gu2019badnets}, the attackers optimize their backdoor attack with respect to $\epsilon$ and $\rho$: $\arg\min_{\epsilon, \rho} f(\theta_{\frac{|X+\epsilon|}{|V|}=\rho} = Y^{*})$.

Following the aforementioned definitions, 
we can unify the attack objectives of both adversarial and backdoor attacks as following attack objective:
% we can reformulate the attacker objectives as the following:

\begin{equation}
\begin{cases}
\min p_s(x+\epsilon) = \min_{\epsilon} \max_{\alpha_s} \alpha_s(\epsilon) \cdot  p_s(\epsilon|t) + (1-\alpha_s(\epsilon)) \cdot p_s(x|s) \\
\max p_t(x+\epsilon) = \min_{\epsilon} \max_{\alpha_t} \alpha_t(\epsilon) \cdot  p_t(\epsilon|t) + (1-\alpha_t(\epsilon)) \cdot p_t(x|s)
\end{cases}
\end{equation}

% \begin{equation}
% \text{\textit{Adversarial attack:} } \min p_s(x+\epsilon) = \min_{\epsilon} \max_{\alpha} \alpha p_s(\epsilon|t) + (1-\alpha)p_s(x|s)
% \end{equation}

% $$\text{\textit{Adversarial attack:} } \min_{\epsilon} \max_{\alpha} p_s(x+\epsilon) = \alpha p_s(\epsilon|t) + (1-\alpha)p_s(x|s)$$

% \begin{equation}
% \text{\textit{Backdoor attack:} } \min p_t(x+\epsilon) = \min_{\epsilon} \max_{\alpha} \alpha p_t(\epsilon|t) + (1-\alpha)p_t(x|s)
% \end{equation}

% $$\text{\textit{Backdoor attack:} } \min_{\epsilon} \max_{\alpha} p_t(x+\epsilon) = \alpha p_t(\epsilon|t) + (1-\alpha)p_t(x|s)$$

where $x \sim {X_i}^{i \in I}_{Y=s}$, 
$\epsilon \sim {X_j}^{j \in J}_{Y=t}$, 
$\alpha_s, \alpha_t \in [0, 1]$,
$s \neq t$.
We reframe the classification of a label by a DNN as evaluating the probability of $x+\epsilon$ belonging to $s$ or $t$ by decomposing $p_{Y}$ into sub-inputs, and evaluating the probability of these sub-inputs belonging to either class. 
Attackers aim to create imperceptible perturbations ($\min \epsilon$) that originate from a target label $t$, either computed with respect to the gradients of the model (adversarial attack) or is known to the attacker from train-time poisoning (backdoor attack). 
$\alpha_s(\epsilon), \alpha_t(\epsilon)$ are re-weighting coefficients; they vary as a function of $\epsilon$, and re-weight the decomposed features and their likelihood of pertaining to a specific class. 
With the introduction of $\epsilon$, attackers hope to $\min p_s(\epsilon|t)$ and $\max p_t(\epsilon|t)$, while $\max \alpha_s(\epsilon), \alpha_t(\epsilon)$, thus reducing the likelihood of $x+\epsilon$ pertaining to classes $s$ and $t$ respectively. 
For $\epsilon \rightarrow 0$, $p_s(x) \approx p_t(x+\epsilon)$, which follows the definition of label shift.

}
